# Supplementary material for: From soft to hard magnetic Fe-Co-B by spontaneous strain: A combined first principle and thin film study
Source: arXiv:1509.04126 source file (2015-09-14)
Supplement: Supplementary file 1 [file Supplementary.pdf]

# Supplemental material for article: "From soft to hard magnetic Fe-Co-B by spontaneous strain: A combined first principle and thin film study"

L. Reichel* and L. Schultz

*IFW Dresden, P.O. Box 270116, 01171 Dresden, Germany and*

*TU Dresden, Faculty of Mechanical Engineering,*

*Institute of Materials Science, 01062 Dresden, Germany*

D. Pohl, S. Oswald, and S. Fähler

*IFW Dresden, P.O. Box 270116, 01171 Dresden, Germany*

M. Werwiński

*Division of Materials Theory, Department of Physics and Astronomy,*

*Uppsala University, Box 516, SE-751 20, Uppsala, Sweden and*

*Institute of Molecular Physics, Polish Academy of Sciences, 60-179 Poznań, Poland*

A. Edström, E. K. Delczeg-Czirjak, and J. Rusz

*Division of Materials Theory, Department of Physics and Astronomy,*

*Uppsala University, Box 516, SE-751 20, Uppsala, Sweden*

## I. OCTAHEDRAL INTERSTITIAL SITES IN A BCC LATTICE

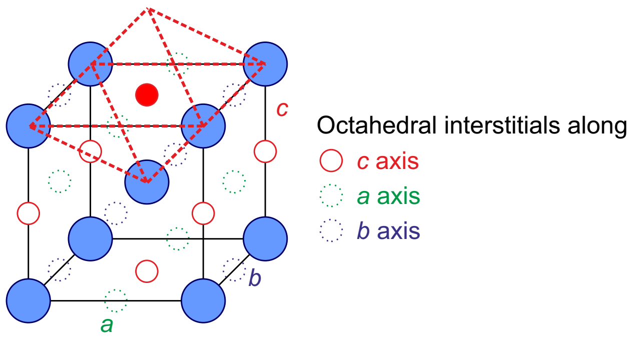


FIG. 1. Location of the octahedral interstitial sites in bcc Fe-Co. with respect to their corresponding axes.

There are six octahedral interstitial sites in a bcc lattice as depicted in Fig. 1. In the image, one exemplary octahedron is sketched for an interstitial, which is located along the $c$ axis. An occupation of an octahedral interstitial by a B atom causes a shift of the atoms on the octahedron's apexes and thus a strain along this particular axis. A preferential occupation of the octahedral sites along the $c$ axis (red circles), as shown in DFT calculations and experiments of our study, results in $c/a > 1$. An additional occupation of the other octahedral interstitial sites (green and blue) decreases the tetragonal strain.

## II. POLE FIGURE MEASUREMENTS

Fig. 2 presents the {011} pole figure of the 20 nm thick $Fe_{0.38}Co_{0.62}$ film with 9.6 at% B. The four poles at $\psi \approx 46°$ and $\phi = 45 + n \cdot 90°$ confirm the epitaxial growth, which holds for all studied B contents in Fe-Co. The shift to higher $\psi$ values is a measure for the tetragonal distortion: $c/a = \tan\psi$. The intensity at $\psi = 0$ originates from the Au-Cu(002) buffer and the MgO(002) substrate poles.

In Fig. 3, a {011} pole figure of a 100 nm thick $Fe_{0.38}Co_{0.62}$ film with 2 at% B is presented. Its tetragonal distortion is $c/a = 1.033 = \tan(45.94°)$, which is identical to the $c/a$ ratio of thinner films with the same composition and thus a strong indication of a spontaneously strained phase.

All measured pole figures confirm the presence of one predominant variant with the strained $c$ axis perpendicular to the film surface.

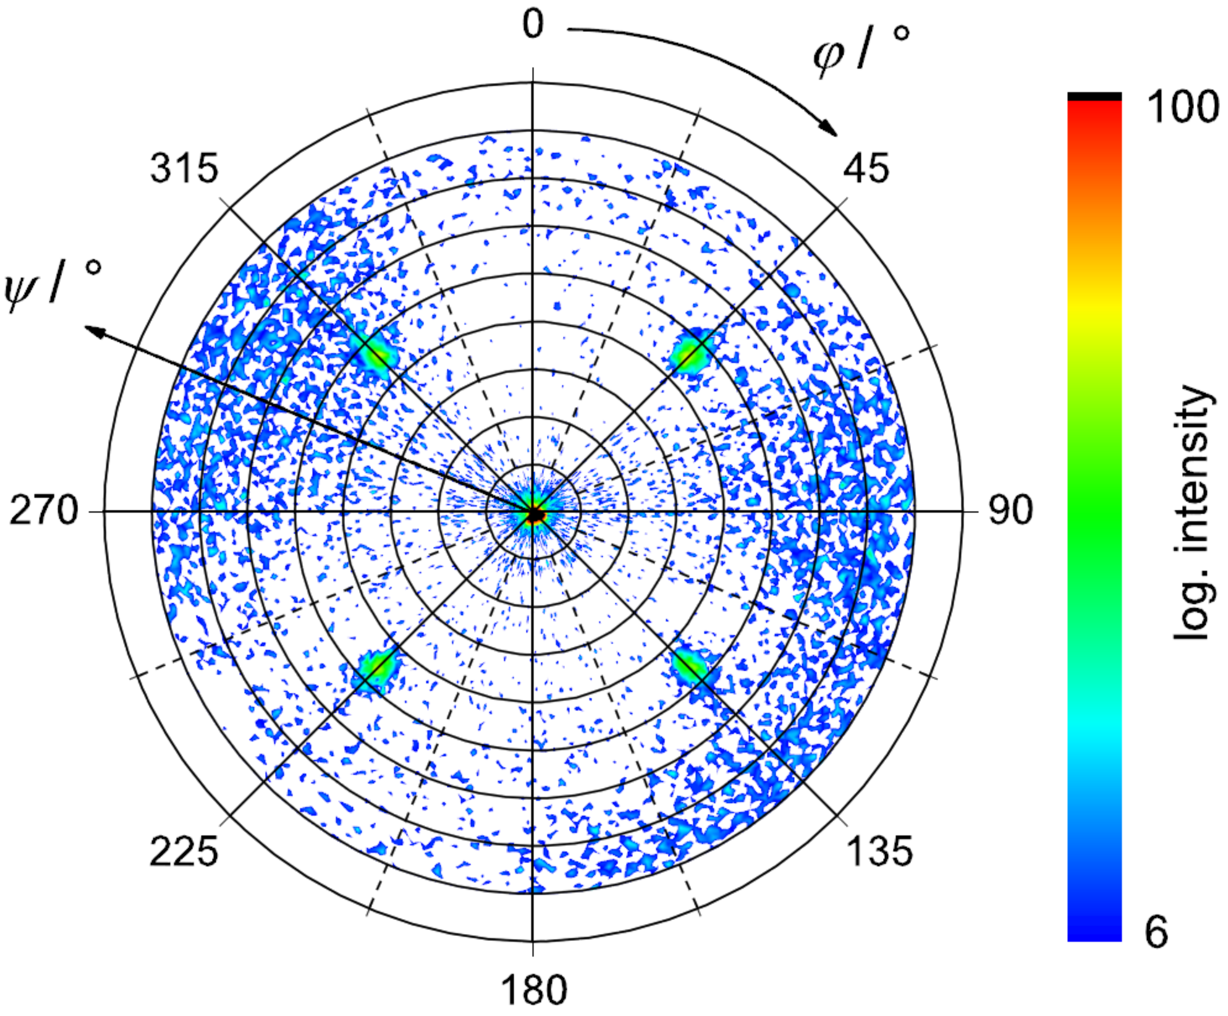


FIG. 2. {011} pole figure of the 20 nm thick $Fe_{0.38}Co_{0.62}$ film with 9.6 at% B.

## III. ADDITIONAL TEM IMAGES

In order to study the influence of the supposed B supersaturation, the $Fe_{0.38}Co_{0.62}$ film with 9.6 at% B was classically thinned for further TEM investigations: After grinding in a isopropanol-glycerin mixture with an Allied Systems Multiprep, the sample was irradiated with $Ar^+$ ions in a PIPS II Gatan, which was equipped with two Penning sources, under an angle of 10° during $LN_2$ cooling. The $Ar^+$ starting acceleration voltage was 3 kV and stepwise reduced ending at 0.2 kV. Fig. 4(a) presents a TEM plane view of this film. The final lamella thickness was determined by measuring the attenuation of the electron beam in the Titan$^3$ 80-300 microscope using the log-ratio method for a given total mean free path for elastic scattering. In the case of Fig. 4(a), it is around 10 nm, which is below the

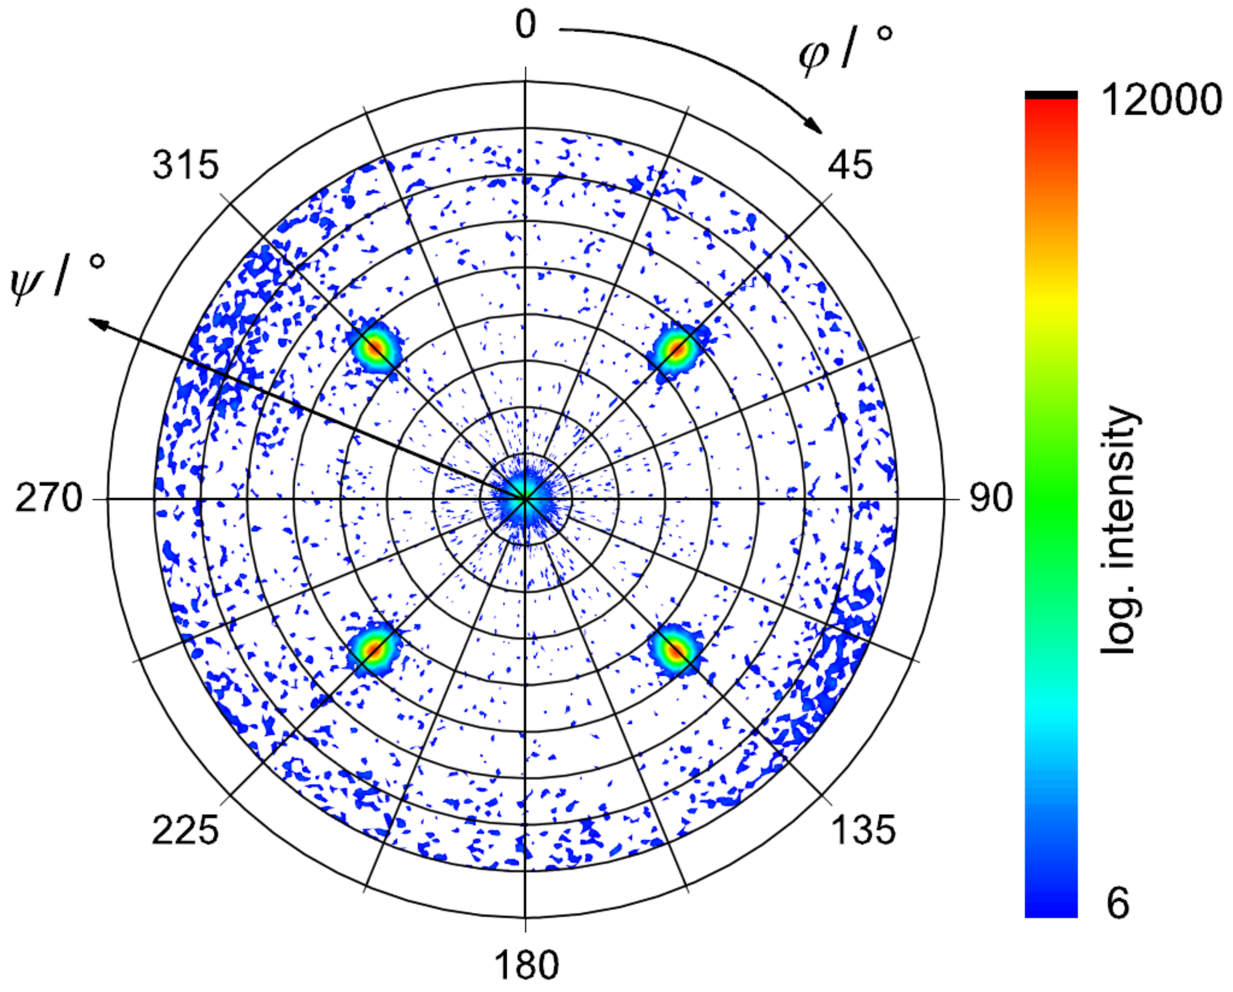


FIG. 3. {011} pole figure of a 100 nm thick $Fe_{0.38}Co_{0.62}$ film with 2 at% B.

film thickness. The Fourier Transform (FT), Fig. 4(b), reveals a superimposition of two nanocrystalline phases with different in-plane lattice parameters, which can be determined as $a_1 = 0.284$ nm and $a_2 = 0.304$ nm from a profile through the FT as shown in Fig. 4(c). Both phases are in epitaxial relationship to the lattice of the MgO(100) substrate (and the Au-Cu buffer), which was confirmed on another (thicker) section of the lamella. Their symmetry in the film's plane is quadratic as determined with the FT.

For further analysis of the two apparent phases, we masked the intensity maxima in the FT (Fig. 4(b)) and constructed inverse FT images (IFT), which show the localization of the two different phases. Fig. 5(a), which is the IFT of the lattice with smaller lattice spacing $a_1$, indicates that this phase forms larger grains, which should give significant intensity in x-ray diffraction. Due to a higher intensity in the FT (Fig. 4(c)) compared to the phase with $a_2$, the

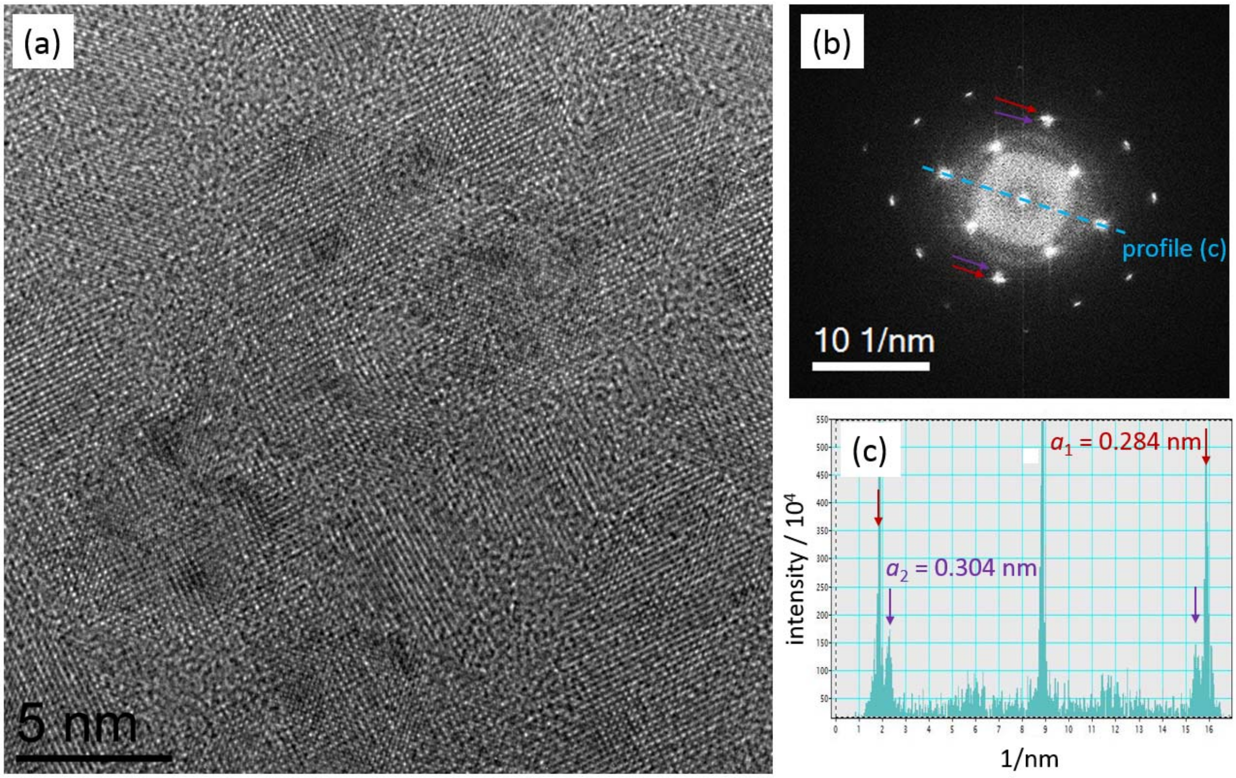


FIG. 4. (a) TEM plane view of the $Fe_{0.38}Co_{0.62}$ film with 9.6 at% B. (b) gives the FT of (a) and. (c) presents the intensity along the profile as already sketched in (b). The intensity maxima originating from two different phases are marked with arrows.

$a_1$ phase is considered as matrix. The IFT of the lattice with the bigger lattice parameter $a_2$ reveals much smaller crystals, mainly with diameters of 2 nm or below. This might explain, why this phase is not detected in XRD. Due to its higher lattice parameter, we argue that this nanocrystalline phase contains more B than the $a_1$ matrix crystals. However, as it appears as nanocrystal precipitates, we do not expect a significant tetragonal strain. Comparing the IFT of the two phases (Fig. 5), we observe regions, where both phases are present, which may indicate that B atoms supersaturating the Fe-Co matrix form the precipitate-like $a_2$ phase very close or within the matrix crystals. In this model, non-crystalline Fe-Co-B should exhibit the highest B content. Such amorphous fractions are visible in Fig. 4(a). Their location coincides with the regions which have no intensity in the IFT (Fig. 5), neither for the $a_1$ nor the $a_2$ phase.

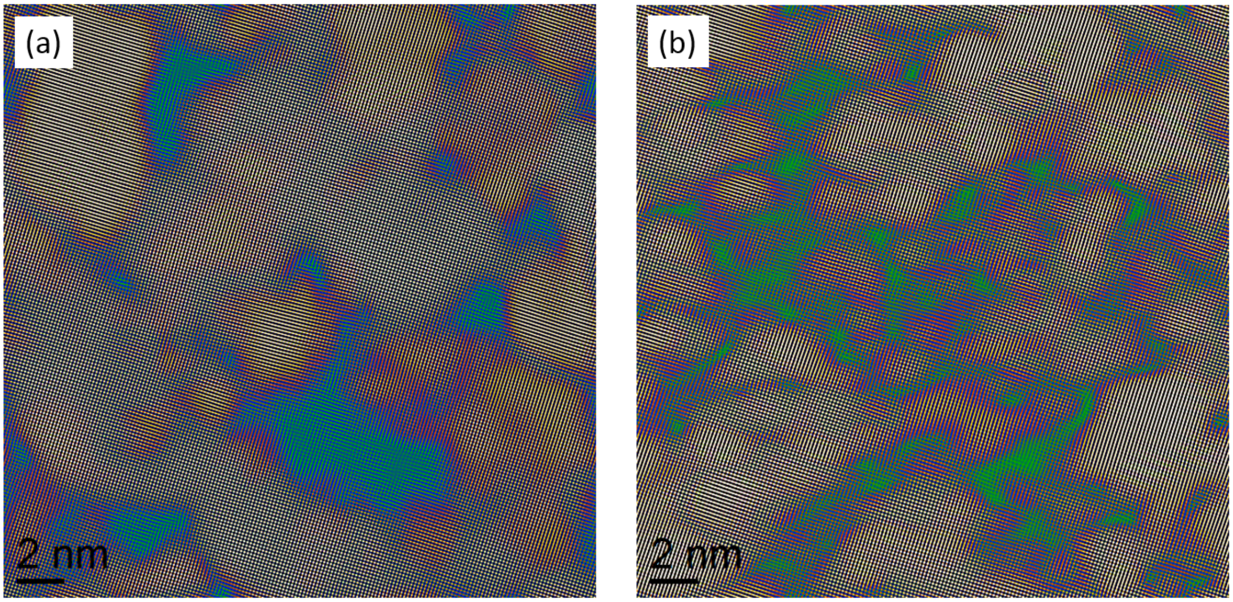


FIG. 5. Inverse FT of Fig. 4(b) with (a) an applied mask for the phase with $a_1 = 0.284\,\mathrm{nm}$ and (b) for the phase with $a_2 = 0.304\,\mathrm{nm}$. Bright regions indicate a high intensity, while greenish or bluish stand for minimum intensity.
